# Supplementary material for: Wideband Modal Orthogonality: A New Approach for Broadband DOA Estimation
Source: arXiv:2006.07261 source file (2020-06-12)
Supplement: Supplementary file 1 [file Appendix1.tex]

\section{Proof of Some Theorems on SO-Transform} \label{sec.app1}
\begin{theorem}
	The SO-Transform for $y_k \in \mathbb{C}$, $k\in\lbrace 0,\cdots , L-1\rbrace$, exists if $y_k$ is absolutely summable.
	\begin{proof}
		\begin{align*}
		\left|Y_{SO^m}(f,\theta)\right| &= \left|\sum_{k} y_k e^{-j2\pi h_k f}\right| \\
		&\le \sum_{k} \left|y_k e^{-j2\pi h_k f}\right| = \sum_{k}\left|y_k\right| < \infty \qedhere
		\end{align*}	
	\end{proof}
\end{theorem}

\begin{theorem}
If the $Y_{SO^m}(f,\theta)$ is absolutely integrable, the inverse SO-Transform exists.
\begin{proof}
	\begin{align*}
	|y_k| &\le \int_{-\infty}^{+\infty} \left|Y_{SO^m}(f,\theta) e^{j2\pi h_k f}\right| \cdot df \\
	&= \int_{-\infty}^{+\infty} \left|Y_{SO^m}(f,\theta)\right| \cdot df \le \infty \qedhere
	\end{align*}
\end{proof}
\end{theorem}

\begin{lemma} \label{lem.sinc}
	The $\text{sinc}(x) = \frac{\sin(ax)}{x}$ behaves as Delta Dirac function, $\delta(x)$, as $a \to \infty$:
	\begin{proof}
		\begin{align*}
		&\left.\int_{-\epsilon}^{+\epsilon} \frac{\sin(ax)}{x} f(x)\cdot dx \right|_{w=ax}
		\int_{-a\epsilon}^{+a\epsilon} \frac{\sin(w)}{w} f(\frac{w}{a})\cdot w
		\end{align*}
		Assuming $f(w)$ a continuous function within $w\in[-\epsilon,+\epsilon]$, then for any $\eta > 0$ there is $\epsilon > 0$ such that $|f(w) - f(0)| < \eta$ then we can replace $f(\frac{w}{a})$ by $f(0)$:
		\begin{align*}
		\int_{-a\epsilon}^{+a\epsilon} \frac{\sin(w)}{w} f(\frac{w}{a})\cdot dw \approx 
		f(0) \int_{-a\epsilon}^{+a\epsilon} \frac{\sin(w)}{w} \cdot dw
		\end{align*}
		for any $\epsilon > 0$ there is a large enough $a$ such that:
		\begin{equation*}
		\int_{-\infty}^{+\infty} \frac{\sin(w)}{w} \cdot dw \to \pi \; as \; a\to \infty
		\end{equation*}
		then:
		\begin{equation*}
		\left.\int_{-\infty}^{+\infty} \frac{\sin(ax)}{x} f(x)\cdot dx \right|_{a\to \infty} = \pi f(0) \qedhere
		\end{equation*}
	\end{proof}
\end{lemma}

\begin{theorem}
	Suppose $y_k$ and $Y_{SO^m}(f,\theta)$ exists, then the inverse SO-Transform exists and converges to $y_k$.
	\begin{proof}
		We start with \eqref{equ.ISOT}:
		\begin{align*}
			y_k &= \int_{-\infty}^{+\infty} Y_{SO^m}(f,\theta) e^{j2\pi h_k f} \cdot df \\
				&= \int_{-\infty}^{+\infty} \left(\sum_{l}y_l e^{-j2\pi h_l f}\right) e^{j2\pi h_k f} \cdot df \\
				&= \lim_{\Omega \to \infty}\sum_{l}y_l \left( \int_{-\Omega/2}^{+\Omega/2} e^{j2\pi (h_k - h_l)f}\cdot df \right) \\
				&= \lim_{\Omega \to \infty}\sum_{l} y_l \frac{\sin(\pi(h_k - h_l)\Omega)}{\pi(h_k - h_l)} = y_k \qedhere
		\end{align*}
		where the last equality obtains from a special discrete time case of Lemma~\ref{lem.sinc}.
		%see Signal Analysis (Roland L.Allen) page 409.
	\end{proof}
\end{theorem}
