# Supplementary material for: Wideband Modal Orthogonality: A New Approach for Broadband DOA Estimation
Source: arXiv:2006.07261 source file (2020-06-12)
Supplement: Supplementary file 2 [file Appendix2.tex]

\section{Semi-Positive Definiteness of $\breve{\mathbf{S}}$, $\breve{\mathbf{S}}^N$ and $\breve{\mathbf{S}}^W$} \label{sec.app2}

%\begin{theorem}
%The matrices $\breve{\mathbf{S}}$, $\breve{\mathbf{S}}^N$ and $\breve{\mathbf{S}}^W$ are positive semi-definite.
%Based on the \textit{Schur product theorem}, the Hadamard product of two positive semidefinite matrices is positive semidefinite\cite{Styan1973}.
\begin{proof}
Matrix $\breve{\mathbf{S}}^N = \mathbf{g}\mathbf{g}^H$  is obviously positive semi-definite. To prove $\breve{\mathbf{S}}^W\succcurlyeq 0$, for an arbitrary nonzero $\mathbf{x}\in \mathbb{C}^L$ we have,
\begin{align*}
\mathbf{x}^H \mathbf{S}^W \mathbf{x} &= \sum_{k,l}x_k^* \frac{\sin(\pi B (h_k - h_l))}{\pi B (h_k - h_l)} x_l\\
& =\sum_{k,l} x_k^* \left(\frac{1}{B}\int_{-B/2}^{+B/2} e^{j2\pi (h_k - h_l)u}\cdot du\right) x_l \\
& =\frac{1}{B} \int_{-B/2}^{+B/2} \left| \sum_{k} x_k e^{-j2\pi h_k u} \right|^2 \cdot du \ge 0
\end{align*}
Finally, the positive-definiteness of the matrix $\breve{\mathbf{S}}$ is derived from the \textit{Schur product theorem}, which states the Hadamard product of two positive semidefinite matrices is positive semidefinite \cite{Styan1973}. %It could also be directly obtained from part~\ref{item.c} of Theorem~\ref{the.1}.
%
%For $\mathbf{S}$ it follows immediately from \eqref{equ.int_approx} that for all nonzero $\mathbf{x}\in \mathbb{C}^L$:
%\begin{align*}
%\mathbf{x}^H \mathbf{S} \mathbf{x} &= \frac{1}{B} \int_{f_1}^{f_2} \mathbf{x}^H\mathbf{g}(u,\theta)\mathbf{g}^H(u,\theta)\mathbf{x} \cdot du \\
%&= \frac{1}{B} \int_{f_1}^{f_2} \left|\mathbf{x}^H\mathbf{g}(u,\theta)\right|^2 \cdot du \ge 0 %
%\end{align*}
\end{proof}
%\end{theorem}
